# Supplementary material for: Practical protein-pocket hydration-site prediction for drug discovery on a quantum computer
Source: arXiv:2512.08390 ancillary file (2025-12-11)
Supplement: Supplementary file 1 [file Supplementary-Information.pdf]

# Supplementary Information for "Practical protein-pocket hydration-site prediction for drug discovery on a quantum computer"

Daniele Loco[1,+], Kisa Barkemeyer[2,+], Andre R. R. Carvalho[2], and Jean-Philip Piquemal[1,3,*]

[1]Qubit Pharmaceuticals, Advanced Research Team, 75014 Paris, France
[2]Q-CTRL, Berlin, Germany and Sydney, NSW Australia
[3]Sorbonne Université, LCT, UMR 7616 CNRS, 75005 Paris, France
[*]Email: jean-philip.piquemal@sorbonne-universite.fr
[+]these authors contributed equally to this work

## 1 Computational workflow for QUBO-based hydration site prediction

We use our own python script to implement the QUBO-base workflow described in the main text. The script implements the steps needed to map the molecular modelling problem onto a Quadratic Unconstrained Binary Optimization (QUBO) form. The script also performs the simulated annealing simulations, using the *neal* library. To perform a QAOA hybrid quantum/classical optimization, the QUBO matrix computed by the script can be saved and later used to feed Q-CTRL's Fire Opal solver. For the notation used, and the details of the QUBO formulation, we refer the reader to the main text. In what follows we present further details of the workflow.

### 1.1 Phase 1: Setup and 3D-RISM Density Processing

The script first pre-process the 3D-RISM density as described in Fig. 9 from the main text, focusing the problem on a selected area of the protein. Then it re-samples it and reduces the problem complexity, generating a grid of variables where the QUBO coefficients are computed.

The following steps are executed by the script:

1. load data: it reads the 3D-RISM density, $g(\mathbf{r})$, from a `.dx` file and loads the coordinates of a reference geometric point user-defined (*vide infra*); for our application this corresponds to a target water cluster.
2. bulk correction: $g(\mathbf{r})$ is corrected by subtracting the bulk water value, focusing on structural correlations: $p(\mathbf{r}) \leftarrow g(\mathbf{r}) - 1$.
3. sub-domain selection: selects a cubic sub-domain, $p(\mathbf{r})$, of the full 3D-RISM grid. The size of this box is determined dynamically to ensure it covers the target water cluster area and accommodates a user-defined number of QUBO variables ($N_{qubo}$).
4. variable's grid generation: the script use the $N_{qubo}$ user-defined to generate the grid of variables used to define and solve the QUBO problem:

(a) it creates qubo variables sites: a cubic lattice of variables sites, $\mathbf{r}_i$, is created. The number of sites is based on $N_{qubo}$.

(b) translate grid: the entire lattice is translated to be centered over the geometric center of a reference water cluster or any pre-defined geometric point user-defined, ensuring the search space aligns with the area of interest, *e.g.*, inside the protein 3D molecular structure.

## 1.2 Phase 2: QUBO Matrix Q Assembly

The QUBO coefficients $Q_{ij}$ are calculated using a model that relates water placement stability to the 3D-RISM density. The model represents a potential water molecule at site $i$ as a normalize Gaussian function $G_i(\mathbf{r})$ centered at $\mathbf{r}_i$ with variance $\sigma^2$. The amplitude $A_i$ of this Gaussian is set by the local density: $A_i = p(\mathbf{r}_i)$. More details about the model and its parameters can be found in the main text and in Section 2 of this Supplementary Materials.

### 1.2.1 QUBO variables filtering

To apply the problem complexity reduction scheme described in the main text (see Methods section, Fig 9, the density $p(\mathbf{r})$ is filtered according to an user-decided threshold $\tau_g$. the script discards any site $\mathbf{r}_i$ where the local density $p(\mathbf{r}_i)$ is below the set threshold ($\tau_g$). This reduces the QUBO dimensionality to only structurally relevant sites.

We remind here, as discussed in the main text, that this step is implemented in the current workflow to reduce the computational cost of both classical and quantum simulations, but it is not a step inherent to the modelling approach we propose.

### 1.2.2 Diagonal coefficients ($Q_{ii}$)

The diagonal term $Q_{ii}$ is seen as the energy cost of placing a single water molecule at site $i$. It has two components, both of which are added to the $Q_{ii}$ element, as:

1. interaction with environment: the interaction with the solvent environment, mediated by $p(\mathbf{r})$) is:

$$Q_{ii}^{(1)} = -2 \int p(\mathbf{r}) G_i(\mathbf{r}) d\mathbf{r} \tag{1}$$

calculated numerically using Simpson's rule.

2. self-interaction: self-interaction energy of the Gaussian density is added analytically as:

$$Q_{ii}^{(2)} = \int G_i(\mathbf{r})^2 d\mathbf{r} \tag{2}$$

this term derives directly from the $L^2$ norm used to derive the QUBO model

### 1.2.3 off-diagonal coefficients ($Q_{ij}, i \neq j$)

The off-diagonal term $Q_{ij}$ are seen as the interaction energy between two water molecules at sites $i$ and $j$. This term is computed analytically taking advantage of the Gaussian functions' properties:

$$Q_{ij} = \int G_i(\mathbf{r}) G_j(\mathbf{r}) d\mathbf{r}. \tag{3}$$

This calculation is parallelized using python multi-processing.

### 1.3 Phase 3: Optimization and Analysis

#### 1.3.1 Optimization

1. QUBO model conversion: the dictionary of coefficients $\mathbf{Q}_{ij}$ is converted to a QUBO model object using the *dimod* library

2. Simulated Annealing: the model is solved using the *neal* library, using 100 sweeps and $10,000$ reads, resulting in a set of low-energy solutions $\mathbf{x}$, which represents here a set of binary strings, each of length $N_{qubo}$, and their associated costs

#### 1.3.2 Result Analysis

1. solution extraction: the script collects all unique solutions and calculates their frequencies.

2. clustering and configuration generation: a dedicated function performs a post-processing step:

   - it identifies the lowest-energy solution (Ground State, GS)
   - for key solutions (including the GS), it extracts the coordinates of all sites where $x_i = 1$; each solution collection of coordinates represents a proposed configuration of hydration sites

3. output writing: the obtained hydration sites configurations are saved , and an analysis plot is generated to visualize the energy distribution of the sampled solutions.

## 2 Grid size and GMM parameters tuning

The QUBO formulation of the GMM problem proceeds by placing a certain number of binary variables in a defined volume of space where a continuous 3D-RISM density is defined. As we described in the previous section, a model 3D gaussian distribution is associated to each variable. For simplicity, we arrange the variables in a regular cubic grid, so that we remain with a number of free parameters, as:

1. the amplitude and variance of the gaussians

2. the spacing of the QUBO grid

The amplitude of each Gaussian is assigned from the value of the underlying 3D-RISM density. For each QUBO variable defined on the grid, the closest point of the 3D-RISM grid is selected. The corresponding value of the 3D-RISM density is assigned as amplitude of the gaussian associated to the QUBO variable. This procedure is repeated for each QUBO variable.

For the gaussian variance and QUBO grid spacing, we tested a few combinations in order to better understand their impact on the problem solution. We report the results in Fig. 1. The metrics described in the section Methods, namely P, C, and $< CS >$, are computed for each water placement, obtained on a single protein of the selected dataset, namely the protein with PDB ID = 1x70.

Each parameter affects the simulation cost and accuracy. For higher values of $\Delta$ a coarser mapping of the density onto the QUBO problem is expected. We tested the impact of this parameter while the variance of the gaussian functions has been fixed to an arbitrary value of 0.8 Å$^2$. Fig. 1, panel a, shows opposite tendencies: P decreases for increasing $\Delta$, while C decreases, together with $< CS >$ since they are connected. The number of placed cluster (C) is the most sensitive metric, dropping from an average of 0.8 to an average of 0.4 for increasing values of $\Delta$. As a consequence around 50% of the clusters identified while using $\Delta = 0.5$ Åare missed in the case where $\Delta = 2.0$ Å.

The change in C is significant because, at least in the extremes of the range of considered $\Delta$, the C values fall outside the 95% interval of confidence (IC). For the other two metrics, the effect seems somehow smaller, and the interval of confidence for $\Delta < 2.0$ Åis large enough to make the differences in the averages fall inside the 95% IC.

The effect of the variance is analyzed in a similar way in Fig. 1, panel b. The grid spacing is set to a value close to the resolution of the 3D-RISM grid (0.5 Å), that is, 0.875 Å. Also in this case the geneal trend is that P increases while C and $< CS >$ decreases for larger values of the gaussian variance. Both P and C change sensibly , ranging from 0.3 to 0.6, and from 0.4 to 0.9, respectively. The differences between the values in the extremes of the tested variances seems statistically relevant considering the 95% IC, in general smaller for the largest variance. The effect of the variance is overall qualitatively the same as that of the $\Delta$ but more pronounced: in both cases, for larger value of the parameter less crystal water are identified by the QUBO, and the fewer identified water are closer to the crystal reference (P and $< CS >$ closer to 1.0)

Therefore, we tested the combination of an average (in the explored range) value of $\Delta$ with an average value of the gaussian variance variance. A set of five combinations is tested, whose parameters are reported in Table 1, and the results are reported in Fig. 2.

| | 1 | 2 | 3 | 4 | 5 |
|---|---|---|---|---|---|
| $\delta$ (Å) | 0.875 | 0.875 | 0.500 | 0.500 | 0.500 |
| $\sigma^2$ (Å$^2$) | 1.00 | 0.80 | 0.80 | 1.00 | 1.00 |
| $\tau_g$ | 0.10 | 0.10 | 0.10 | 0.10 | 0.05 |

Table 1: Set of parameters used to compute the metrics reported in Fig. 2; each triad of parameters is label with an integer value, reported in the header of the table

## 3 List of classical methods for hydration sites prediction

In Tab. 2 we list the classical methods, not based on a QUBO formulation, we used for the benchmarking performed in this work. The table reports limited details on each method. A full description of each method can be found in the related cited bibliography.

## 4 Details on comparison with classical methods

Here we report the list of additional test used to asses the QUBO-based method's performance.

To expand and discuss in more details the scale-up analysis discussed in the Results section of the main text, we report in Fig. 3 additional results using PDB ID = 3beq from Tab. 1 in the main text. We include both results obtained with the Q-CTRL solver on the IBM quantum device and classical Simulated Annealing (SA) results, for instances encompassing more than 156 variables.

As we already observed in the main text, the smaller instances are able to recover already a good portions of the reference crystal water (CW) positions, in this case up to 80% of CWs (8 of the 10 present in the crystal structure). For the largest problem sizes (more than 1000 variables), P*, C and <CS> show a notable increase. In particular <CS> exceed the value of 1.0. This is explained by the fact that geometrically extended regions of higher density are

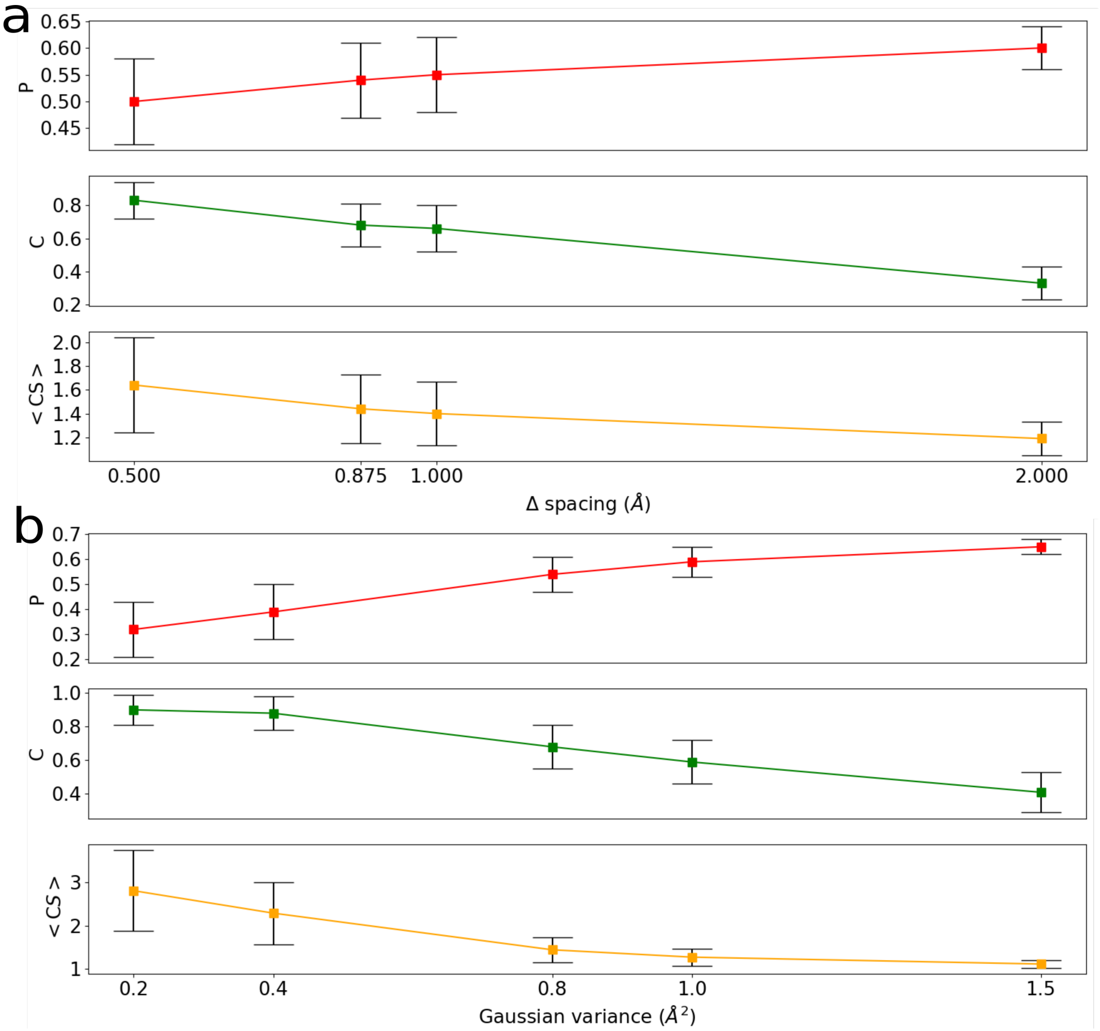


Figure 1: Metrics, and respective 95% interval of confidence, evaluated on the chosen test case (PDB ID: 1x70): a) varying values of the grid spacing; the grid spacing is reported as values on the x-axis of the graphs.b) varying values of the gaussian variance; the variance value is reported as value on the x-axis of the graphs; all metrics, defined in the Methods section of the main text, are evaluated on the best solution found from a SA simulation, using the *neal* library, a geometric scheduling for the temperature and sampling the solutions 10,000 times

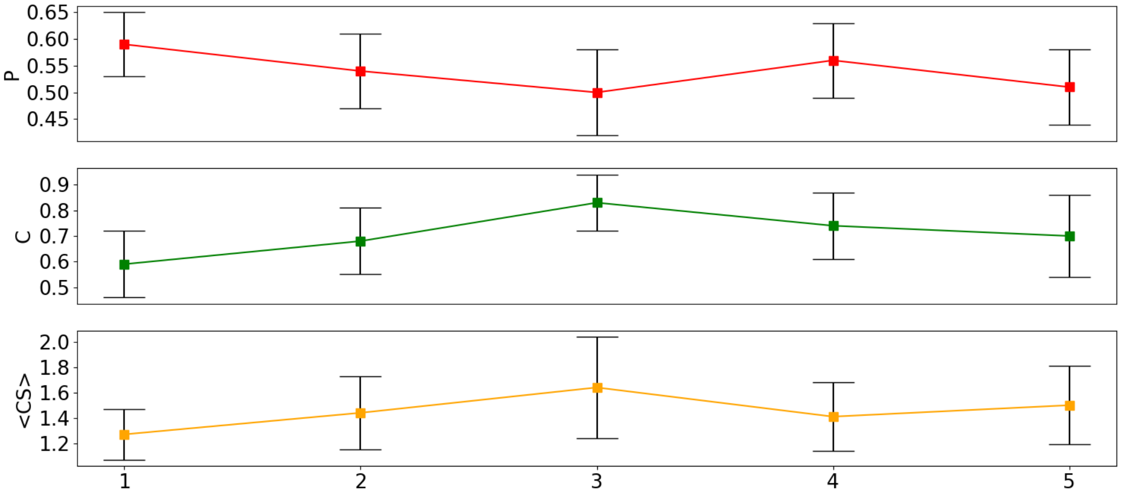


Figure 2: Metrics results obtained for the chosen test case (PDB ID: 1x70) with a set of parameters as defined in Tab. 1; the x-axis reports the integers, used to label the choice for the triad of parameters used to define the QUBO problem; all metrics are evaluated on the best solution found from a SA simulation, using the *neal* library, a geometric scheduling for the temperature and sampling the solutions 10,000 times

| Software | Class | Benchmark dataset | Description |
|---|---|---|---|
| Placevent | Interaction-based site prediction | 2 | Takes a 3D-RISM density as input and places water molecules in its maxima, vacating at each iteration an area around the placed water molecule. |
| HydraProt | Deep learning | “full” PDB | Works in three stages: first a 3D U-net is used to process the atomic coordinates of a protein to find a large set of possible water molecule positions, then a MLP evaluates each candidate water molecule, and then a final step refines the solution by applying a fixed set of rules. |
| WaterKit | Interaction-based site prediction | 7 | grid-based sampling method with explicit water molecules based on the Grid Inhomogeneous Solvation Theory (GIST) design to compute thermodynamic properties of water molecules for high-throughput pipelines. The hydration sites are extracted from the GIST's oxygen density, iteratively selecting the region with highest densities, imposing a minimal distance of 2.5 Å [1] |
| WATGEN | Knowledge-based | 9000 | Water site prediction on the basis of experimentally observed geometries of hydration around amino acids. A binding site is flooded with water, then the sites forming the best interactions with the protein are kept, removing any clashes. |
| Dowser++ | Interaction-based site prediction | 16 | Water molecules are inserted into cavities and optimised, before keeping/discarding sites based on interaction energy. The Dowser method first minimises the water molecules and each is kept if the interaction energy is sufficiently negative. |

Table 2: List of software used in this work to compare the QUBO model performance; the definition of the class to which each method belongs is taken from the literature [2, 3]

mapped by more the one variable for QUBO grid with small enough spacing. Nevertheless despite a ∼38 fold increase in the problem size, passing from 56 to 2154 variable, only a ∼3 fold increase in placed water is observed.

<P> and <CS> both have an associated statistical variance, which we report as the 95% confidence interval. From Fig. 3 we see how the variability of <P>, quantified by the size of the confidence interval, consistently decrease with the system size. We can observe the same general trend in the additional results we discuss later in this section. This trend is not that clearly followed by <CS>. To support this observation we also report their coefficients of variation in Tab. 3, computed as the ratio between the standard deviation and the mean value of the computed metrics. We can conclude that the prediction becomes more robust for larger instances, since the variability of <P> tends to become lower while its average value increases.

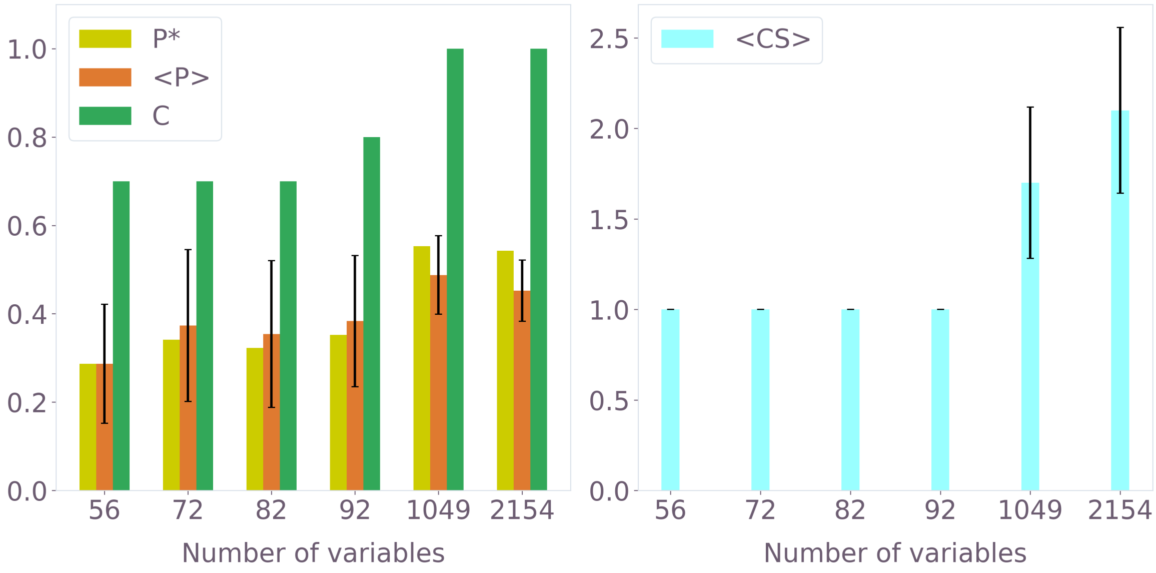


Figure 3: Analysis of the hydration-sites prediction performance across different QUBO instance sizes for PDB ID = 3beq from Tab. 1 in the main text. The number of variables used for each instance is noted on the x-axis. The instance with 72 variables corresponds to system m in Tab 2. P* (closest water placement precision, light blue), <P> (cluster-averaged precision, orange) and C (fraction of crystal waters identified, green) are presented on the left-side plot; <CS> (average cluster size, violet) is showed on the center plot. Error bars show the 95% confidence interval for <P> and <CS>. Each metric is computed as described in the Methods section, extracting the PWs corresponding to the best solution obtained: using the Q-CTRL solver on the IBM Kingston device for instances from 56 to 92 variables, and the classical SA for instances with 1049 and 2154 variables. The following parameters have been used to compute the QUBO matrices, starting from the smaller instance toward the larger one: a gaussian variance $\sigma^2 = 1.0\ \text{Å}^2$ is used uniformly, density values lower than $\tau_g = 0.11, 0.11, 0.1, 0.09$ and 0.05, respectively, are ignored to reduce the problem sizes, while $\delta = 1.27, 1.15, 1.15, 1.15$, and 0.5 Å are used to discretize the the computed 3D-RISM density

Four additional cases are reported in Fig. 4, corresponding to PDB IDs = 1f9g with ligand, 3b7e without ligand and 4h2f with and without ligand, respectively. Observing the behavior of the metrics with the increasing of the QUBO complexity, we can enforce the observation discussed in the previous paragraphs and in the main text.

From Fig. 4 we can in fact observe that: increasing size and complexity of the QUBO problem, the hydration-site prediction gains in accuracy; the actual optimal size of the QUBO instance depends on the specific density. For system

| # variables | CV(<P>) | CV(<CS>) |
|---|---|---|
| 56 | 0.76 | 0.0 |
| 72 | 0.74 | 0.0 |
| 82 | 0.75 | 0.0 |
| 92 | 0.62 | 0.0 |
| 1049 | 0.29 | 0.4 |
| 2154 | 0.25 | 0.3 |

Table 3: Coefficients of variations for PDB ID = 3brq in Fig. 3, computed as the ratio between the standard deviation and the mean value of <P> and <CS>, respectively

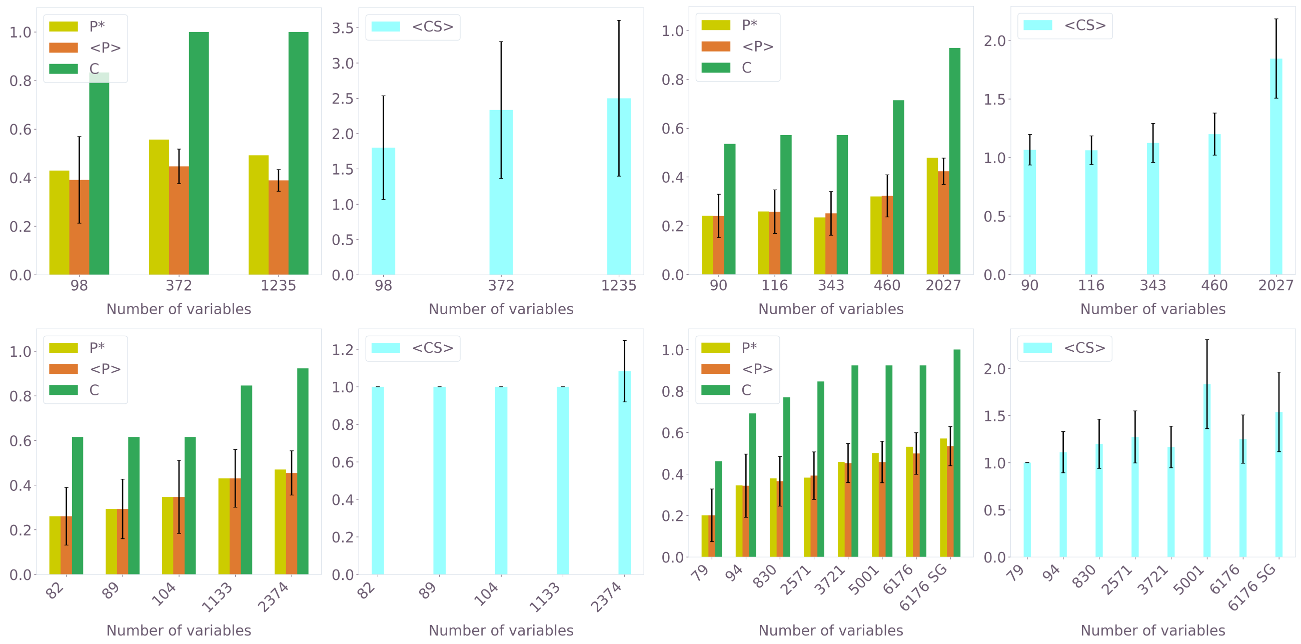


Figure 4: Performance and variability across different size instances of QUBO for, in the order: PDB IDs = 1f9g with ligand (top left), 3b7e without ligand (top right), 4h2f with ligand (bottom left) and without ligand (bottom right). P* (closest water placement precision, light blue), <P> (cluster-averaged precision, orange) and C (fraction of crystal waters identified, green) are presented on the left-side plot; <CS> (average cluster size, violet) is showed on the center plot. Error bars show the 95% confidence interval for <P> and <CS>.

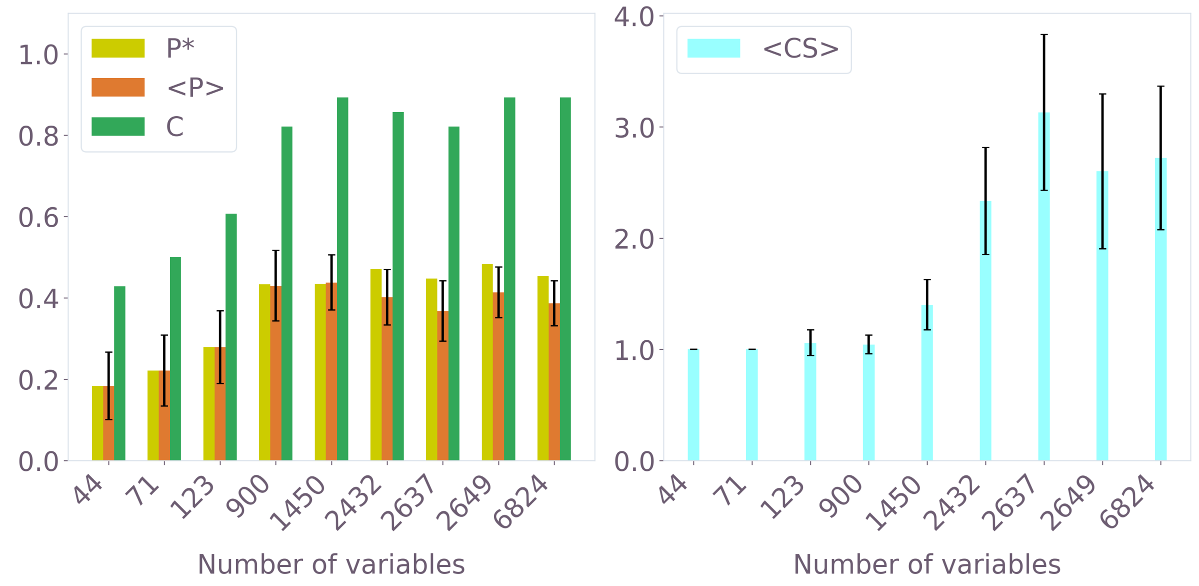


Figure 5: Performance and variability across different sizes of QUBO instances for PDB ID = 3b7e (see Tab. 1 in the main text), including the ligand in the 3D-RISM calculation. The number of variables used for each instance is noted on the x-axis. P* (closest water placement precision, light blue), <P> (cluster-averaged precision, orange) and C (fraction of crystal waters identified, green) are presented on the left-side plot; <CS> (average cluster size, violet) is showed on the center plot. Error bars show the 95% confidence interval for <P> and <CS>. Each metric is computed as described in the Methods section, extracting the PWs corresponding to the best solution obtained: using the Q-CTRL solver on the IBM Kingston device for instances from 44 to 123 variables, and the classical SA for all the larger instances. The instance with 71 variables, corresponds to system g in Tab. 2, while the 123 instance has been analysed in the main text, Fig. 3 . For all instances, a gaussian variance $\sigma^2 = 1.0$ $\textbf{Å}^2$ as been used, while the rest of the model parameters used, $\tau_g$ and $\delta$ are reported in Tab. 4

| # variables | CV(<P>) | CV(<CS>) | $\tau_g$ | $\delta$ ( **Å**) |
|---|---|---|---|---|
| 44 | 1.22 | 0.00 | 0.10 | 1.35 |
| 71 | 1.06 | 0.00 | 0.10 | 1.15 |
| 123 | 0.86 | 0.23 | 0.10 | 0.95 |
| 900 | 0.54 | 0.20 | 0.10 | 0.5 |
| 1450 | 0.42 | 0.41 | 0.05 | 0.5 |
| 2432 | 0.46 | 0.51 | 0.006 | 0.5 |
| 2637 | 0.54 | 0.55 | 0.0006 | 0.5 |
| 2649 | 0.41 | 0.68 | 0.0003 | 0.5 |
| 6824 | 0.39 | 0.60 | 0.0002 | 0.35 |

Table 4: Coefficients of variations (CV) for a series of QUBO instances computed from PDB ID = 3b7e (see Tab. 1 in the main text) including the ligand in the 3D-RISM calculation; the instance with 71 variables corresponds to system g in Tab. 2 in the main text; CV is computed as the ratio between the standard deviation and the mean value of <P> and <CS>, respectively; we also reported the parameters used to compute the respective QUBO instances; a uniform $\sigma^2 = 1.0\text{Å}^2$ is used

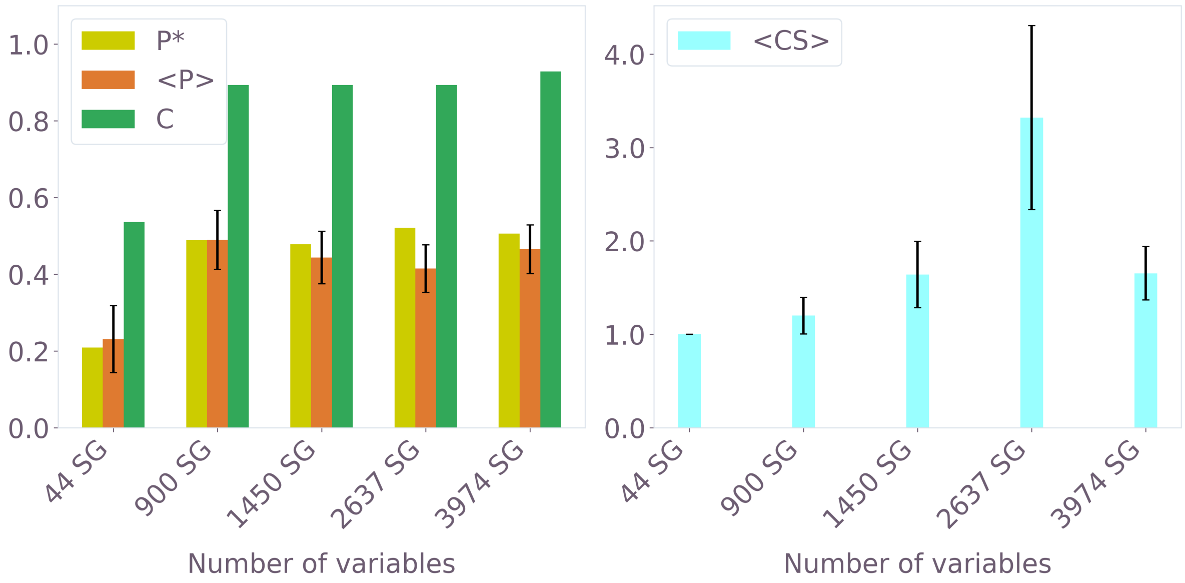


Figure 6: Performance and variability across different sizes of QUBO instances for PDB ID = 3b7e (see Tab. 1 in the main text), including the ligand in the 3D-RISM calculation. The number of variables used for each instance is noted on the x-axis. P* (closest water placement precision, light blue), <P> (cluster-averaged precision, orange) and C (fraction of crystal waters identified, green) are presented on the left-side plot; <CS> (average cluster size, violet) is showed on the center plot. Error bars show the 95% confidence interval for <P> and <CS>. Each metric is computed as described in the Methods section, extracting the PWs corresponding to the best solution obtained using classical SA for all instances. For all instances, a smaller gaussian (SG) variance $\sigma^2 = 0.8$ $\text{Å}^2$ as been used, while the rest of the model parameters, $\tau_g$ and $\delta$ are reported in Tab. 5

| # variables | CV(<P>) | CV(<CS>) |
|---|---|---|
| 44 SG | 1.02 | 0.00 |
| 900 SG | 0.42 | 0.42 |
| 1450 SG | 0.42 | 0.55 |
| 2637 SG | 0.40 | 0.76 |
| 3974 SG | 0.37 | 0.45 |

Table 5: Coefficients of variations (CV) for a series of QUBO instances computed from PDB ID = 3b7e (see Tab. 1 in the main text) including the ligand in the 3D-RISM calculation; SG stands for smaller gaussian, since here $\sigma^2 = 0.8\text{Å}^2$; CV is computed as the ratio between the standard deviation and the mean value of <P> and <CS>, respectively

| # variables | CV(<P>) | CV(<CS>) |
|---|---|---|
| 98 | 0.57 | 0.46 |
| 372 | 0.20 | 0.52 |
| 1235 | 0.14 | 0.55 |

Table 6: Coefficients of variations for PDB ID = 1f9g with ligand; it is computed as the ratio between the standard deviation and the mean value of <P> and <CS>, respectively

| # variables | CV(<P>) | CV(<CS>) |
|---|---|---|
| 90 | 1.00 | 0.24 |
| 116 | 0.94 | 0.23 |
| 343 | 0.96 | 0.30 |
| 460 | 0.72 | 0.34 |
| 2027 | 0.34 | 0.48 |

Table 7: Coefficients of variations for PDB ID = 3b7e without ligand; it is computed as the ratio between the standard deviation and the mean value of <P> and <CS>, respectively

| # variables | CV(<P>) | CV(<CS>) |
|---|---|---|
| 82 | 0.91 | 0.00 |
| 89 | 0.84 | 0.00 |
| 104 | 0.87 | 0.00 |
| 1133 | 0.55 | 0.00 |
| 2374 | 0.40 | 0.27 |

Table 8: Coefficients of variations for PDB ID = 4h2f with ligand; it is computed as the ratio between the standard deviation and the mean value of <P> and <CS>, respectively

| # variables | CV(<P>) | CV(<CS>) |
|---|---|---|
| 79 | 1.17 | 0.00 |
| 94 | 0.81 | 0.30 |
| 830 | 0.60 | 0.35 |
| 2571 | 0.54 | 0.37 |
| 3721 | 0.38 | 0.33 |
| 5001 | 0.40 | 0.45 |
| 6176 | 0.37 | 0.36 |
| 6176 SG | 0.32 | 0.50 |

Table 9: Coefficients of variations forPDB ID = 4h2f without ligand; it is computed as the ratio between the standard deviation and the mean value of <P> and <CS>, respectively

| # variables | CV(<P>) | CV(<CS>) |
|---|---|---|
| 6176 | 0.37 | 0.36 |
| 6176 SG | 0.32 | 0.50 |
| Hydraprot | 0.33 | 0.41 |
| Placevent | 1.69 | 0.00 |
| Watgen | 0.11 | 0.42 |
| Waterkit | 0.65 | 0.44 |

Table 10: Coefficients of variations for PDB ID = 4h2f without ligand, comparing QUBO and classical approaches; it is computed as the ratio between the standard deviation and the mean value of <P> and <CS>, respectively

1f9g with ligand, we reach good performances already at 372 variables. as reported in Fig. 1, this is the case with the smaller water network size, between the selected system. For all the three other cases reported, passing from ∼100 to ∼1000 variables increase considerably the accuracy of the prediction quality, as testify by a steep increase of C and the general improvement of both P and <P>.

In Fig. 5 we further expand the analysis reported in the main text on the case of PDB ID = 3b7e with ligand included in the 3D-RISM calculation, encompassing,a larger variety of QUBO instances compared to those shown in the main text (see Fig. 5 there). This is the same system used in the resources forecasting for the scaling-up of the problem, discussed in the Result section in the main text. From the metrics reported in Fig. 5, we can again observe how increasing the QUBO complexity (all model parameters are reported in Tab. 4) the performance metrics generally improve. A sharp improvement is observed when transitioning from 123 to 900 variables, while a limited improvement is observed from 900 to 1450. Moreover, the <CS> metric instance shis negligibly affected by increasing the QUBO size up to 900 variables. On the opposite <CV> noticeably worsen (both its average and confidence interval increase) from 1450. Most remarkably, the 2649 variables instance shows the best performances in terms of P and C. <CS> reaches a plateau after 2432 variables.. We can state then that around 900 variables we can locate the lower-bound to the utility regime that we forecast in the main text.

We show in Fig. 7 an additional comparison with other classical methods not based on the QUBO formulation, using PDB ID = 4h2f without ligand (see Tab. 1 in the main text). This is the same example that we used for the quantum resources forecast. Once again, As observed in the main text, the QUBO-based method largely overperforms Placevent that also uses the 3D-RISM density to find hydration sites. On the other hand Hydraprot shows a non-negligible better (∼15%) score in the accuracy in the identification of the crystal water location. As QUBO, also Hydraprot does not find all the crystal water locations (C < 1.0) and the two methods perform similarly in this regard.

# 5 Local solver results

We report in Tab. 11 the differences between the optimal solution cost and the one found by the local solver ($\Delta_{\text{cost}}(\text{LS})$), which we discussed in the main text in the Results section. As the table shows, for some problem instances the LS fails to find the optimal solution. This is not the case for the Q-CTRL solver and SA

| Test Case | $\Delta_{\text{cost}}(\text{LS})$ |
|---|---|
| a(98) | 0.024128 |
| b(91) | 0.811314 |
| c(69) | 0.000000 |
| d(116) | 9.194522 |
| e(41) | 0.000000 |
| f(92) | 0.570788 |
| g(71) | 0.000000 |
| h(90) | 0.000000 |
| i(82) | 0.000000 |
| l(79) | 1.257258 |

Table 11: List of local solver (LS) best solution cost gaps with respect to the optimal solution costs found for the list of tested systems

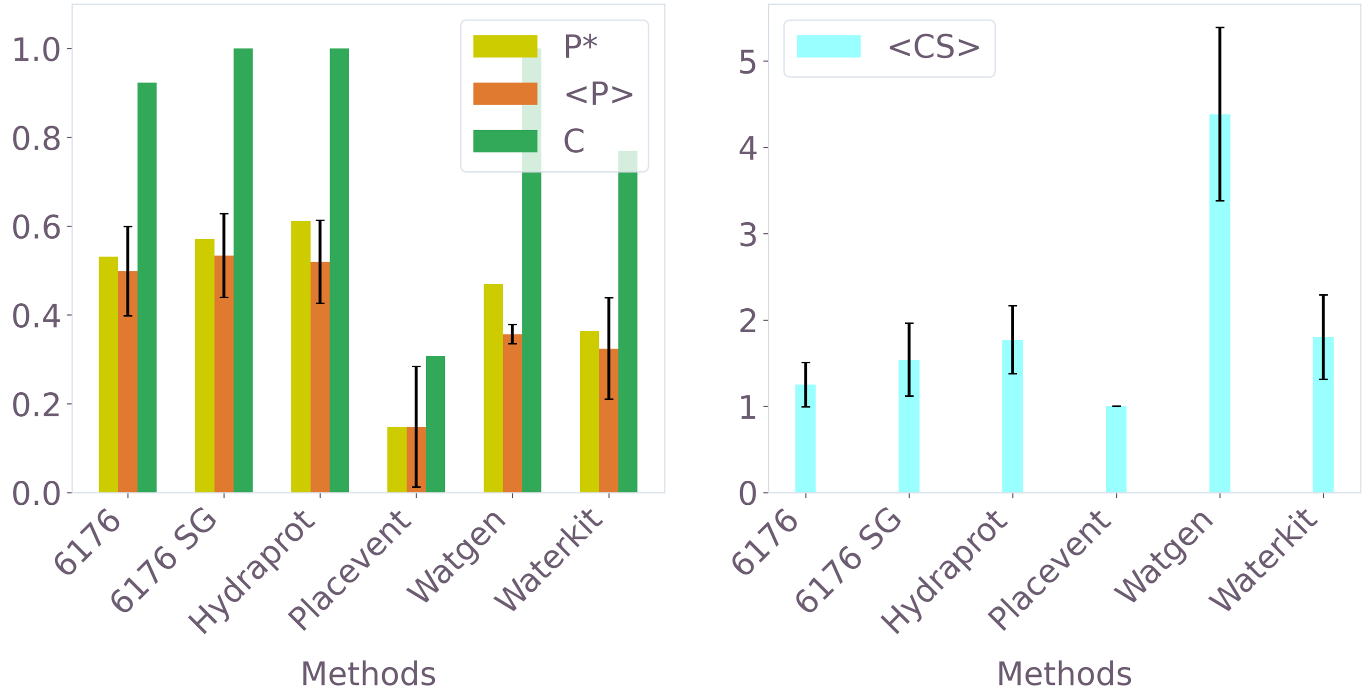


Figure 7: Comparative analysis between the best performing QUBO instance and classical hydration-sites prediction methods, for PDB ID = 4h2f (see Tab. 1 in the main text), without ligand included in the 3D-RISM calculation. The number of variables, and the model parameters used to formulate the QUBO problem, are reported as label on the x-axis. We compare the QUBO-based method with Hydraprot, Watgen, Placevent and Waterkit (see Tab. 2. The figure presents the four performance metrics: P* (closest water placement precision), <P> (cluster-averaged precision), C (fraction of crystal waters identified) are presented on the left plot; <CS> (average cluster size) are showed on the right plot. Error bars show the 95% confidence interval for <P> and <CS>.

# References


[1] Jerome Eberhardt and Stefano Forli. “WaterKit: Thermodynamic Profiling of Protein Hydration Sites”. In: *J. Chem. Theory and Comput.* 19.9 (2023), pp. 2535–2556.

[2] Marley L. Samways et al. “Water molecules at protein–drug interfaces: computational prediction and analysis methods”. In: *Chem. Soc. Rev.* 50 (16 2021), pp. 9104–9120.

[3] Eva Nittinger et al. “Placement of Water Molecules in Protein Structures: From Large-Scale Evaluations to Single-Case Examples”. In: *Journal of Chemical Information and Modeling* 58.8 (2018), pp. 1625–1637.
